# Supplementary material for: Semi-Supervised Video Salient Object Detection Using Pseudo-Labels
Source: arXiv:1908.04051 source file (2019-11-29)
Supplement: Supplementary file 1 [file ICCV19_RCRNet_Saliency-supp.pdf]

# Semi-Supervised Video Salient Object Detection Using Pseudo-Labels
## (Supplemental Materials)

Pengxiang Yan[1] Guanbin Li[1*] Yuan Xie[1,2]
Zhen Li[3] Chuan Wang[4] Tianshui Chen[1,2] Liang Lin[1,2]
[1]Sun Yat-sen University [2]DarkMatter AI Research [4]Megvii Technology
[3]Shenzhen Research Institute of Big Data, the Chinese University of Hong Kong (Shenzhen)
yanpx@mail2.sysu.edu.cn, liguanbin@mail.sysu.edu.cn, xiey39@mail2.sysu.edu.cn,
lizhen36@connect.hku.hk, wangchuan@megvii.com, tianshuichen@gmail.com, linliang@ieee.org

## 1. More Comparison with State-of-the-Art

We compare our video saliency model (RCRNet+NER) against 16 state-of-the-art image/video saliency methods, including MC [3], RBD [20], MB+ [19], RFCN [14], DCL [6], DHS [8], DSS [2], MSR [4], DGRL [15], PiCA [9], SAG [16], GF [17], SSA [7], FCNS [18], FGRN [5], and PDB [13]. A more detailed quantitative comparison of maximum F-measure, S-measure, weighted F-measure, and mean absolute error (MAE) on VOS [7], DAVIS [12] and FBMS [1] datasets is presented in Table 1. The weighted F-measure is proposed in [10] to mitigate the interpolation flaw, dependency flaw, and equal-importance flaw of traditional evaluation metrics. Here, we use the code provided by the authors with the default setting. MAE is defined as the average absolute difference between the binary ground truth and the saliency map at the pixel level [11]. As shown in Table 1, our method outperforms all existing salient object detection algorithms across all datasets. Specifically, our method improves the maximum F-measure achieved by the existing best-performing algorithms by 15.52%, 1.18%, and 4.62% respectively on VOS, DAVIS, and FBMS, and improves the S-measure by 9.41%, 0.68%, 2.72% accordingly. Moreover, our method improves the weighted F-measure by 17.04%, 3.23%, and 3.68% respectively on VOS, DAVIS, and FBMS, and reduces the MAE by 34.67%, 6.67%, and 5.26% accordingly.

## 2. Sensitivities to Different Amount of Ground Truth and Pseudo-Labels Usage

To demonstrate the effectiveness of our proposed semi-supervised framework, we explore the sensitivities to different amount of ground truth and pseudo-labels usage on the VOS [7] dataset. We fine-tune our proposed video saliency detector RCRNet+NER with different number of GT and pseudo-labels. Detailed quantitative results on the test set of VOS are presented in Table 2. As seen, models cannot generate temporally consistent saliency maps when the training data set is seriously deficient (e.g., 5%) , which results in inferior performance. Nevertheless, an interesting phenomenon is that when there are enough training data with similar appearance, given more annotation data does not guarantee continuous performance improvement. This phenomenon may be due to model overfitting caused by label ambiguity. Based on the above observations, we propose jointly training RCRNet+NER with an appropriate number of pseudo-labels (e.g., 20%) and GT labels (e.g., 20%). Experimental results demonstrate the effectiveness of using pseudo-labels for training. Moreover, our semi-supervised RCRNet+NER (column '1 / 5' in the table) can even outperform the one trained with all annotated frames.

*Corresponding author is Guanbin Li.

## References

[1] Thomas Brox and Jitendra Malik. Object segmentation by long term analysis of point trajectories. In *Proceedings of European Conference on Computer Vision*, pages 282–295, 2010. 1, 2

[2] Qibin Hou, Ming-Ming Cheng, Xiaowei Hu, Ali Borji, Zhuowen Tu, and Philip HS Torr. Deeply supervised salient object detection with short connections. In *Proceedings of IEEE Conference on Computer Vision and Pattern Recognition*, pages 3203–3212, 2017. 1, 2

[3] Bowen Jiang, Lihe Zhang, Huchuan Lu, Chuan Yang, and Ming-Hsuan Yang. Saliency detection via absorbing markov chain. In *Proceedings of the IEEE International Conference on Computer Vision*, pages 1665–1672, 2013. 1, 2

[4] Guanbin Li, Yuan Xie, Liang Lin, and Yizhou Yu. Instance-level salient object segmentation. In *Proceedings of IEEE Conference on Computer Vision and Pattern Recognition*, pages 2386–2395, 2017. 1, 2

| | Methods | Pub. | VOS [7] | | | | DAVIS [12] | | | | FBMS [1] | | | |
|---|---|---|---|---|---|---|---|---|---|---|---|---|---|---|
| | | | $F_\beta^{max}\uparrow$ | $S\uparrow$ | $F_\beta^w\uparrow$ | MAE$\downarrow$ | $F_\beta^{max}\uparrow$ | $S\uparrow$ | $F_\beta^w\uparrow$ | MAE$\downarrow$ | $F_\beta^{max}\uparrow$ | $S\uparrow$ | $F_\beta^w\uparrow$ | MAE$\downarrow$ |
| I+C | MC [3] | CVPR'13 | 0.558 | 0.612 | 0.306 | 0.199 | 0.488 | 0.590 | 0.201 | 0.182 | 0.466 | 0.567 | 0.251 | 0.237 |
| | RBD [20] | CVPR'14 | 0.589 | 0.652 | 0.419 | 0.148 | 0.481 | 0.620 | 0.264 | 0.142 | 0.488 | 0.591 | 0.307 | 0.194 |
| | MB+ [19] | ICCV'15 | 0.577 | 0.638 | 0.401 | 0.167 | 0.520 | 0.568 | 0.231 | 0.229 | 0.540 | 0.586 | 0.319 | 0.244 |
| I+D | RFCN [14] | ECCV'16 | 0.680 | 0.721 | 0.499 | 0.108 | 0.732 | 0.788 | 0.514 | 0.069 | 0.764 | 0.765 | 0.563 | 0.108 |
| | DCL [6] | CVPR'16 | 0.704 | 0.728 | 0.551 | 0.086 | 0.760 | 0.803 | 0.578 | 0.065 | 0.760 | 0.772 | 0.630 | 0.088 |
| | DHS [8] | CVPR'16 | 0.715 | 0.783 | 0.611 | **0.075** | 0.785 | 0.820 | **0.662** | **0.040** | 0.765 | 0.793 | 0.671 | 0.083 |
| | DSS [2] | CVPR'17 | 0.703 | 0.760 | 0.587 | 0.082 | 0.775 | 0.814 | 0.621 | 0.056 | 0.776 | 0.793 | 0.656 | 0.083 |
| | MSR [4] | CVPR'17 | 0.719 | 0.764 | 0.599 | 0.102 | 0.775 | 0.789 | 0.589 | 0.065 | 0.809 | 0.835 | 0.709 | 0.067 |
| | DGRL [15] | CVPR'18 | 0.723 | 0.776 | 0.622 | **0.079** | 0.758 | 0.811 | 0.652 | 0.058 | 0.813 | 0.834 | **0.761** | **0.057** |
| | PiCA [9] | CVPR'18 | **0.734** | **0.796** | **0.633** | 0.090 | **0.809** | **0.844** | 0.660 | 0.044 | **0.823** | **0.847** | 0.730 | **0.058** |
| V+U | SAG [16] | CVPR'15 | 0.541 | 0.597 | 0.309 | 0.178 | 0.519 | 0.663 | 0.329 | 0.107 | 0.545 | 0.632 | 0.345 | 0.176 |
| | GF [17] | TIP'15 | 0.529 | 0.560 | 0.318 | 0.264 | 0.619 | 0.686 | 0.374 | 0.094 | 0.609 | 0.642 | 0.365 | 0.172 |
| | SSA [7] | TIP'18 | 0.669 | 0.710 | 0.580 | 0.117 | 0.697 | 0.738 | 0.601 | 0.068 | 0.597 | 0.634 | 0.496 | 0.165 |
| V+D | FCNS [18] | TIP'18 | 0.681 | 0.727 | 0.439 | 0.125 | 0.764 | 0.757 | 0.407 | 0.091 | 0.752 | 0.747 | 0.475 | 0.129 |
| | FGRN [5] | CVPR'18 | 0.714 | 0.734 | 0.547 | 0.082 | 0.797 | 0.838 | 0.662 | 0.044 | 0.801 | 0.818 | 0.643 | 0.083 |
| | PDB [13] | ECCV'18 | **0.741** | **0.797** | **0.632** | 0.080 | **0.849** | **0.878** | **0.744** | **0.030** | **0.823** | **0.839** | **0.732** | 0.067 |
| | Ours* | ICCV'19 | **0.856** | **0.872** | **0.776** | **0.049** | **0.859** | **0.884** | **0.768** | **0.028** | **0.861** | **0.870** | **0.789** | **0.054** |

* Note that our model is a semi-supervised learning model using only about 20% ground truth labels for training.

Table 1. Comparison of quantitative results using maximum F-measure $F_\beta^{max}$ (larger is better), S-measure $S$ (larger is better), weighted F-measure $F_\beta^w$ (larger is better), and MAE (smaller is better). The best three results on each dataset are shown in **red**, **blue**, and **green**, respectively. Symbols of model categories: I+C for image-based classic unsupervised or non-deep learning methods, I+D for image-based deep learning methods, V+U for video-based unsupervised methods, V+D for video-based deep learning methods.

| Labels | $m$ / $l$ | 0 / 1 | 0 / 2 | 0 / 3 | 2 / 3 | 0 / 5 | 1 / 5 | 2 / 5 | 4 / 5 | 0 / 7 | 1 / 7 | 2 / 7 | 6 / 7 |
|---|---|---|---|---|---|---|---|---|---|---|---|---|---|
| Proportion | GT | 100% | 50% | 33.3% | 33.3% | 20% | 20% | 20% | 20% | 14.3% | 14.3% | 14.3% | 14.3% |
| | Pseudo | 0% | 0% | 0% | 0% | 0% | 20% | 40% | 80% | 0% | 14.3% | 28.6% | 85.7% |
| Metric | $F_\beta^{max}\uparrow$ | 0.849 | 0.850 | 0.852 | 0.851 | 0.849 | **0.861** | 0.851 | 0.850 | 0.847 | 0.856 | 0.851 | 0.846 |
| | $S\uparrow$ | 0.873 | 0.869 | 0.873 | 0.873 | 0.867 | **0.874** | 0.869 | 0.873 | 0.866 | 0.872 | 0.869 | 0.867 |

| Labels | $m$ / $l$ | 0 / 10 | 2 / 10 | 3 / 10 | 9 / 10 | 0 / 15 | 4 / 15 | 5 / 15 | 14 / 15 | 0 / 20 | 6 / 20 | 7 / 20 | 19 / 20 |
|---|---|---|---|---|---|---|---|---|---|---|---|---|---|
| Proportion | GT | 10% | 10% | 10% | 10% | 6.7% | 6.7% | 6.7% | 6.7% | 5% | 5% | 5% | 5% |
| | Pseudo | 0% | 20% | 30% | 90% | 0% | 26.7% | 33.3% | 93.3% | 0% | 30% | 35% | 95% |
| Metric | $F_\beta^{max}\uparrow$ | 0.839 | 0.859 | 0.850 | 0.849 | 0.823 | 0.849 | 0.851 | 0.849 | 0.821 | 0.847 | 0.847 | 0.845 |
| | $S\uparrow$ | 0.861 | 0.872 | 0.868 | 0.867 | 0.842 | 0.866 | 0.868 | 0.865 | 0.832 | 0.861 | 0.861 | 0.860 |

Table 2. More quantitative results on different amount of ground truth (GT) and pseudo-labels usage. Here, $l$ refers to GT label interval, and $m$ denotes the number of pseudo-labels used in each interval. For example, '0 / 5' means using one GT every five frames with no pseudo-labels. '1 / 5' means using one GT and generating one pseudo-label every five frames. And so on.


[5] Guanbin Li, Yuan Xie, Tianhao Wei, Keze Wang, and Liang Lin. Flow guided recurrent neural encoder for video salient object detection. In *Proceedings of IEEE Conference on Computer Vision and Pattern Recognition*, pages 3243–3252, 2018. 1, 2

[6] Guanbin Li and Yizhou Yu. Deep contrast learning for salient object detection. In *Proceedings of IEEE Conference on Computer Vision and Pattern Recognition*, pages 478–487, 2016. 1, 2

[7] Jia Li, Changqun Xia, and Xiaowu Chen. A benchmark dataset and saliency-guided stacked autoencoders for video-based salient object detection. *IEEE Transactions on Image Processing*, 27(1):349–364, 2018. 1, 2

[8] Nian Liu and Junwei Han. Dhsnet: Deep hierarchical saliency network for salient object detection. In *Proceedings of IEEE Conference on Computer Vision and Pattern Recognition*, pages 678–686, 2016. 1, 2

[9] Nian Liu, Junwei Han, and Ming-Hsuan Yang. Picanet: Learning pixel-wise contextual attention for saliency detection. In *Proceedings of IEEE Conference on Computer Vision and Pattern Recognition*, pages 3089–3098, 2018. 1, 2

[10] Ran Margolin, Lihi Zelnik-Manor, and Ayellet Tal. How to evaluate foreground maps? In *Proceedings of IEEE Conference on Computer Vision and Pattern Recognition*, pages 248–255, 2014. 1

[11] Federico Perazzi, Philipp Krähenbühl, Yael Pritch, and Alexander Hornung. Saliency filters: Contrast based filtering for salient region detection. In *Proceedings of IEEE Conference on Computer Vision and Pattern Recognition*, pages 733–740, 2012. 1

[12] Federico Perazzi, Jordi Pont-Tuset, Brian McWilliams, Luc Van Gool, Markus Gross, and Alexander Sorkine-Hornung. A benchmark dataset and evaluation methodology for video object segmentation. In *Proceedings of IEEE Conference on Computer Vision and Pattern Recognition*, pages 724–732, 2016. 1, 2

[13] Hongmei Song, Wenguan Wang, Sanyuan Zhao, Jianbing Shen, and Kin-Man Lam. Pyramid dilated deeper convlstm for video salient object detection. In *Proceedings of European Conference on Computer Vision*, pages 715–731, 2018. 1, 2

[14] Linzhao Wang, Lijun Wang, Huchuan Lu, Pingping Zhang, and Xiang Ruan. Saliency detection with recurrent fully convolutional networks. In *Proceedings of European Conference on Computer Vision*, pages 825–841, 2016. 1, 2

[15] Tiantian Wang, Lihe Zhang, Shuo Wang, Huchuan Lu, Gang Yang, Xiang Ruan, and Ali Borji. Detect globally, refine locally: A novel approach to saliency detection. In *Proceedings of IEEE Conference on Computer Vision and Pattern Recognition*, pages 3127–3135, 2018. 1, 2

[16] Wenguan Wang, Jianbing Shen, and Fatih Porikli. Saliency-aware geodesic video object segmentation. In *Proceedings of IEEE Conference on Computer Vision and Pattern Recognition*, pages 3395–3402, 2015. 1, 2

[17] Wenguan Wang, Jianbing Shen, and Ling Shao. Consistent video saliency using local gradient flow optimization and global refinement. *IEEE Transactions on Image Processing*, 24(11):4185–4196, 2015. 1, 2

[18] Wenguan Wang, Jianbing Shen, and Ling Shao. Video salient object detection via fully convolutional networks. *IEEE Transactions on Image Processing*, 27(1):38–49, 2018. 1, 2

[19] Jianming Zhang, Stan Sclaroff, Zhe Lin, Xiaohui Shen, Brian Price, and Radomir Mech. Minimum barrier salient object detection at 80 fps. In *Proceedings of the IEEE International Conference on Computer Vision*, pages 1404–1412, 2015. 1, 2

[20] Wangjiang Zhu, Shuang Liang, Yichen Wei, and Jian Sun. Saliency optimization from robust background detection. In *Proceedings of IEEE Conference on Computer Vision and Pattern Recognition*, pages 2814–2821, 2014. 1, 2
